# Supplementary material for: Counting Stacked Objects
Source: arXiv:2411.19149 source file (2025-07-30)
Supplement: Supplementary file 1 [file supp_real_samples.tex]

\newcommand{\names}{beans,chickpeas,chocolates,crosses,crosses2,gums2,popcorn,puzzle,screws,screws2,semicrosses,semicrosses2}

\newcommand{\counts}{161,2668,201,40,317,500,2229,574,295,627,156,196}
\newcommand{\gts}{207,3276,131,205,205,397,2921,1000,514,494,257,257}

\begin{figure}[ht]
    \centering
    % Top row with RGB images and input names
    %\foreach \input in \inputnames {%
    \foreach \name [count=\j from 0] in \names {
        \pgfmathparse{array({\counts},{\j})} % Extract the j-th count
        \edef\count{\pgfmathresult}
        \pgfmathparse{array({\gts},{\j})} % Extract the j-th count
        \edef\gt{\pgfmathresult}
        \begin{minipage}[c]{0.32\linewidth} % Adjust width for spacing
            \centering
            %\textbf{\input} \vspace{0.2em} \\ % Input name at the top of each column
            %\includegraphics[width=\textwidth]{images/samples/00000392_RGB.png}
            \includegraphics[width=\textwidth]{images/supp_real/\name.jpg}
            \vspace{-2em}\caption*{\centering\textit{\name}:\\\textit{Est.} \count,  \\\textit{G.T.} \gt}\vspace{0.5em}
        \end{minipage}\hspace{-0.5em}%
    }

    \caption{\textbf{Additional dataset samples.} We report the results on all real scenes that are not already present in our main submission.}
    \label{fig:additional_real_samples}
\end{figure}

\iffalse

DOUBLE COLUMN 

\begin{figure*}[ht]
    \centering
    % Top row with RGB images and input names
    %\foreach \input in \inputnames {%
    \foreach \name [count=\j from 0] in \names {
        \pgfmathparse{array({\counts},{\j})} % Extract the j-th count
        \edef\count{\pgfmathresult}
        \pgfmathparse{array({\gts},{\j})} % Extract the j-th count
        \edef\gt{\pgfmathresult}
        \begin{minipage}[c]{0.23\textwidth} % Adjust width for spacing
            \centering
            %\textbf{\input} \vspace{0.2em} \\ % Input name at the top of each column
            %\includegraphics[width=\textwidth]{images/samples/00000392_RGB.png}
            \includegraphics[width=\textwidth]{images/supp_real/\name.jpg}
            \vspace{-2em}\caption*{\centering\textit{\name}:\\\textit{Est.} \count,  \textit{G.T.} \gt}\vspace{1em}
        \end{minipage}%
    }

    \caption{\textbf{Additional dataset samples.} We report the results on all real scenes that are not already present in our main submission.}
    \label{fig:additional_real_samples}
\end{figure*}

\fi
